# Supplementary material for: Qubit Mapping and Routing via MaxSAT
Source: arXiv:2208.13679 source file (2022-08-29)
Supplement: Supplementary file 1 [file 9Appendix.tex]

\section{Key Modifications}
All modifications are in \diff{blue} text. We summarize the three key revisions
requested below.

\paragraph{1. Scalability vs. Optimality}
We added a new research question (Q5) that investigates the scalability–optimality tradeoff. 
Specifically, \cref{fig:cost_vs_timeout} shows how increasing the time limit produces better and better solutions, stagnating at $\sim$4000 seconds and circuits with $\sim$1700 two-qubit gates. 
Since we don't have the ground truth for the optimal answer, we compare our solutions to \tket on circuits of increasing size (\cref{fig:tket_cost_vs_size}). As expected, we notice that on larger circuits the cost ratio converges to ~1, since the local relaxation requires more slices. Note that \nisq algorithms are expected to have \#s of two-qubit gates in the low 100s, and our evaluation goes well beyond that.

\paragraph{2. Source of Improvements} We expand Q3 to clearly indicate the source of improvement. Specifically, \cref{table:olsq_vs_us} shows that every algorithmic decision in the paper almost doubles the number of solvable circuits, starting with \olsq as the strong baseline. \textbf{It is important to note that \olsq outperforms Triq [Murali et al. 2019, citation 22 in revision] on scalability and optimality -- as per \olsq paper and our independent corroboration -- and so we use \olsq as our state-of-the-art baseline.}
\begin{itemize}
    
    \item Without relaxations, \nolocal can solve 70 benchmarks, while \olsq only 38. This is due to our new encoding: While the number of constraints is roughly the same as \olsq (see analysis in \cref{sec:alg}), \textbf{our sketch-based view of the mapping and routing problem allows us to eschew the use of integer arithmetic, eliminating the expensive theory-lemma generation of an \smt solver.}
    \item With local relaxation, \ours can solve 109 benchmarks, with a largest circuit of size 598, compared to \olsq's largest circuit size solved of 90.
    \item We also see the same behavior in \qaoa benchmarks, with the local relaxation and cyclic relaxations allowing us to solve progressively more benchmarks. Indeed, \olsq is unable to solve any of our \qaoa benchmarks within the allotted time.
\end{itemize}

\paragraph{3. Noise-Aware \qmr}
We added a new research question (Q6) that addresses noise models. We modified our implementation to handle gate fidelities, using weighted \maxsat to maximize probability (in a similar fashion to TB-OLSQ). We used the fidelity data from \textsc{ibm} Tokyo in Qiskit. The results vs \olsq are analogous to those in Q2, with \ours solving $\sim$4x more benchmarks.
